# Supplementary material for: Mapping Election Polarization and Competitiveness using Election Results
Source: arXiv:2308.10862 source file (2024-07-27)
Supplement: Supplementary file 1 [file Between-EPI-current.tex]

\begin{table}
\begin{center}
\begin{tabular}{l c c c c c c c c c}
\hline
 & Model 1 & Model 2 & Model 3 & Model 4 & Model 5 & Model 6 & Model 7 & Model 8 & Model 9 \\
\hline
Between-EP (t - 1)            & $0.74^{***}$ &          &          &            &          &             &             & $0.71^{***}$ & $0.72^{***}$ \\
                              & $(0.07)$     &          &          &            &          &             &             & $(0.08)$     & $(0.08)$     \\
Inequality level (t)          &              & $-0.23$  &          &            &          &             & $-0.30$     & $-0.01$      & $-0.01$      \\
                              &              & $(0.29)$ &          &            &          &             & $(0.29)$    & $(0.12)$     & $(0.12)$     \\
Unemployment (t)              &              &          & $0.07$   &            &          &             &             & $0.18$       & $0.18$       \\
                              &              &          & $(0.61)$ &            &          &             &             & $(0.23)$     & $(0.23)$     \\
Spatial Between-EP (t)        &              &          &          & $0.08^{*}$ &          &             &             & $0.02$       & $0.02$       \\
                              &              &          &          & $(0.05)$   &          &             &             & $(0.02)$     & $(0.03)$     \\
Ed. Attainment (t)            &              &          &          &            & $0.15$   &             &             &              & $0.02$       \\
                              &              &          &          &            & $(0.26)$ &             &             &              & $(0.12)$     \\
Log of personal Income PC (t) &              &          &          &            &          & $0.26^{*}$  & $0.27^{**}$ & $0.09$       & $0.09$       \\
                              &              &          &          &            &          & $(0.14)$    & $(0.14)$    & $(0.06)$     & $(0.07)$     \\
Log of GDP PC (t)             & $0.01$       & $-0.01$  & $-0.01$  & $0.01$     & $-0.03$  & $-0.18^{*}$ & $-0.19^{*}$ & $-0.04$      & $-0.04$      \\
                              & $(0.02)$     & $(0.04)$ & $(0.05)$ & $(0.05)$   & $(0.07)$ & $(0.10)$    & $(0.10)$    & $(0.04)$     & $(0.04)$     \\
Log of Pop. Density (t)       & $-0.00$      & $0.01$   & $0.01$   & $0.01$     & $0.01$   & $0.00$      & $0.00$      & $-0.00$      & $-0.00$      \\
                              & $(0.00)$     & $(0.01)$ & $(0.01)$ & $(0.01)$   & $(0.01)$ & $(0.01)$    & $(0.01)$    & $(0.00)$     & $(0.00)$     \\
\hline
Num. obs.                     & $250$        & $300$    & $300$    & $300$      & $300$    & $300$       & $300$       & $250$        & $250$        \\
R$^2$ (full model)            & $0.62$       & $0.15$   & $0.15$   & $0.17$     & $0.15$   & $0.19$      & $0.20$      & $0.62$       & $0.62$       \\
R$^2$ (proj model)            & $0.57$       & $0.03$   & $0.02$   & $0.05$     & $0.03$   & $0.07$      & $0.09$      & $0.58$       & $0.58$       \\
Adj. R$^2$ (full model)       & $0.61$       & $0.13$   & $0.12$   & $0.15$     & $0.13$   & $0.17$      & $0.18$      & $0.61$       & $0.60$       \\
Adj. R$^2$ (proj model)       & $0.56$       & $0.00$   & $-0.01$  & $0.02$     & $-0.00$  & $0.04$      & $0.06$      & $0.56$       & $0.56$       \\
Num. groups: year             & $5$          & $6$      & $6$      & $6$        & $6$      & $6$         & $6$         & $5$          & $5$          \\
\hline
\multicolumn{10}{l}{\scriptsize{$^{***}p<0.01$; $^{**}p<0.05$; $^{*}p<0.1$}}
\end{tabular}
\caption{State-level regression analyses of Between-EP as dependent variable. Each regression includes period-fixed effects. Standard errors in brackets. Note: ***$p<0.01$, **$p<0.05$, *$p<0.1$.}
\label{tab:between_epi_2}
\end{center}
\end{table}
