# Supplementary material for: Mapping Election Polarization and Competitiveness using Election Results
Source: arXiv:2308.10862 source file (2024-07-27)
Supplement: Supplementary file 2 [file Between-EPI-v2.tex]

\begin{table}
\begin{center}
\begin{tabular}{l c c c c c c c c}
\hline
 & Model 1 & Model 2 & Model 3 & Model 4 & Model 5 & Model 6 & Model 7 & Model 8 \\
\hline
Inequality level (t - 1)          & $-0.17$  &          &          &          &          & $-0.19$  & $-0.32$     & $-0.31$     \\
                                  & $(0.31)$ &          &          &          &          & $(0.30)$ & $(0.29)$    & $(0.27)$    \\
Unemployment (t - 1)              &          & $0.57$   &          &          &          &          & $1.30^{**}$ & $1.31^{**}$ \\
                                  &          & $(0.65)$ &          &          &          &          & $(0.58)$    & $(0.57)$    \\
Spatial Between-EP (t - 1)        &          &          & $0.06$   &          &          &          & $0.10^{**}$ & $0.10^{**}$ \\
                                  &          &          & $(0.05)$ &          &          &          & $(0.04)$    & $(0.04)$    \\
Ed. Attainment (t - 1)            &          &          &          & $0.16$   &          &          &             & $0.06$      \\
                                  &          &          &          & $(0.18)$ &          &          &             & $(0.32)$    \\
Log of personal Income PC (t - 1) &          &          &          &          & $0.05$   & $0.05$   & $0.12$      & $0.11$      \\
                                  &          &          &          &          & $(0.07)$ & $(0.07)$ & $(0.08)$    & $(0.14)$    \\
Log of GDP PC (t - 1)             & $0.00$   & $-0.00$  & $0.00$   & $0.00$   & $0.00$   & $0.00$   & $-0.00$     & $-0.00$     \\
                                  & $(0.01)$ & $(0.01)$ & $(0.01)$ & $(0.01)$ & $(0.01)$ & $(0.01)$ & $(0.01)$    & $(0.01)$    \\
Log of Pop. Density (t - 1)       & $0.00$   & $0.01$   & $0.00$   & $0.00$   & $0.00$   & $0.00$   & $-0.00$     & $-0.00$     \\
                                  & $(0.01)$ & $(0.01)$ & $(0.01)$ & $(0.01)$ & $(0.01)$ & $(0.01)$ & $(0.01)$    & $(0.01)$    \\
\hline
Num. obs.                         & $250$    & $250$    & $250$    & $250$    & $250$    & $250$    & $250$       & $250$       \\
R$^2$ (full model)                & $0.12$   & $0.13$   & $0.13$   & $0.13$   & $0.13$   & $0.13$   & $0.19$      & $0.19$      \\
R$^2$ (proj model)                & $0.02$   & $0.02$   & $0.03$   & $0.02$   & $0.02$   & $0.03$   & $0.09$      & $0.09$      \\
Adj. R$^2$ (full model)           & $0.10$   & $0.10$   & $0.11$   & $0.10$   & $0.10$   & $0.10$   & $0.15$      & $0.15$      \\
Adj. R$^2$ (proj model)           & $-0.01$  & $-0.01$  & $0.00$   & $-0.01$  & $-0.01$  & $-0.00$  & $0.05$      & $0.05$      \\
Num. groups: year                 & $5$      & $5$      & $5$      & $5$      & $5$      & $5$      & $5$         & $5$         \\
\hline
\multicolumn{9}{l}{\scriptsize{$^{***}p<0.01$; $^{**}p<0.05$; $^{*}p<0.1$}}
\end{tabular}
\caption{State-level regression analyses of Between-EP as dependent variable. Each regression includes period-fixed effects. Standard errors in brackets. Note: ***$p<0.01$, **$p<0.05$, *$p<0.1$.}
\label{tab:between_epi_3}
\end{center}
\end{table}
