# Supplementary material for: Mapping Election Polarization and Competitiveness using Election Results
Source: arXiv:2308.10862 source file (2024-07-27)
Supplement: Supplementary file 3 [file Between-EPI.tex]

\begin{table}
\begin{center}
\begin{tabular}{l c c c c c c c c c}
\hline
 & Model 1 & Model 2 & Model 3 & Model 4 & Model 5 & Model 6 & Model 7 & Model 8 & Model 9 \\
\hline
Between-EP (t - 1)                & $0.74^{***}$ &          &          &          &          &          &          & $0.74^{***}$ & $0.74^{***}$ \\
                                  & $(0.07)$     &          &          &          &          &          &          & $(0.08)$     & $(0.08)$     \\
Inequality level (t - 1)          &              & $-0.17$  &          &          &          &          & $-0.19$  & $0.02$       & $0.05$       \\
                                  &              & $(0.31)$ &          &          &          &          & $(0.30)$ & $(0.09)$     & $(0.10)$     \\
Unemployment (t - 1)              &              &          & $0.57$   &          &          &          &          & $1.02^{***}$ & $1.04^{***}$ \\
                                  &              &          & $(0.65)$ &          &          &          &          & $(0.31)$     & $(0.33)$     \\
Spatial Between-EP (t - 1)        &              &          &          & $0.06$   &          &          &          & $0.01$       & $0.01$       \\
                                  &              &          &          & $(0.05)$ &          &          &          & $(0.02)$     & $(0.02)$     \\
Ed. Attainment (t - 1)            &              &          &          &          & $0.16$   &          &          &              & $0.21$       \\
                                  &              &          &          &          & $(0.18)$ &          &          &              & $(0.13)$     \\
Log of personal Income PC (t - 1) &              &          &          &          &          & $0.05$   & $0.05$   & $0.05$       & $0.00$       \\
                                  &              &          &          &          &          & $(0.07)$ & $(0.07)$ & $(0.03)$     & $(0.05)$     \\
Log of GDP PC (t - 1)             & $0.00$       & $0.00$   & $-0.00$  & $0.00$   & $0.00$   & $0.00$   & $0.00$   & $-0.00$      & $-0.00$      \\
                                  & $(0.00)$     & $(0.01)$ & $(0.01)$ & $(0.01)$ & $(0.01)$ & $(0.01)$ & $(0.01)$ & $(0.00)$     & $(0.00)$     \\
Log of Pop. Density (t - 1)       & $-0.00$      & $0.00$   & $0.01$   & $0.00$   & $0.00$   & $0.00$   & $0.00$   & $-0.00$      & $-0.00$      \\
                                  & $(0.00)$     & $(0.01)$ & $(0.01)$ & $(0.01)$ & $(0.01)$ & $(0.01)$ & $(0.01)$ & $(0.00)$     & $(0.00)$     \\
\hline
Num. obs.                         & $250$        & $250$    & $250$    & $250$    & $250$    & $250$    & $250$    & $250$        & $250$        \\
R$^2$ (full model)                & $0.62$       & $0.12$   & $0.13$   & $0.13$   & $0.13$   & $0.13$   & $0.13$   & $0.64$       & $0.64$       \\
R$^2$ (proj model)                & $0.57$       & $0.02$   & $0.02$   & $0.03$   & $0.02$   & $0.02$   & $0.03$   & $0.59$       & $0.60$       \\
Adj. R$^2$ (full model)           & $0.60$       & $0.10$   & $0.10$   & $0.11$   & $0.10$   & $0.10$   & $0.10$   & $0.62$       & $0.62$       \\
Adj. R$^2$ (proj model)           & $0.56$       & $-0.01$  & $-0.01$  & $0.00$   & $-0.01$  & $-0.01$  & $-0.00$  & $0.57$       & $0.58$       \\
Num. groups: year                 & $5$          & $5$      & $5$      & $5$      & $5$      & $5$      & $5$      & $5$          & $5$          \\
\hline
\multicolumn{10}{l}{\scriptsize{$^{***}p<0.01$; $^{**}p<0.05$; $^{*}p<0.1$}}
\end{tabular}
\caption{State-level regression analyses of Between-EP as dependent variable. Each regression includes period-fixed effects. Standard errors in brackets. Note: ***$p<0.01$, **$p<0.05$, *$p<0.1$.}
\label{tab:between_epi_1}
\end{center}
\end{table}
