# Supplementary material for: Mapping Election Polarization and Competitiveness using Election Results
Source: arXiv:2308.10862 source file (2024-07-27)
Supplement: Supplementary file 4 [file EPI-current.tex]

\begin{table}
\begin{center}
\begin{tabular}{l c c c c c c c c c}
\hline
 & Model 1 & Model 2 & Model 3 & Model 4 & Model 5 & Model 6 & Model 7 & Model 8 & Model 9 \\
\hline
EP (t - 1)                    & $0.72^{***}$ &          &          &          &          &          &          & $0.70^{***}$ & $0.69^{***}$ \\
                              & $(0.05)$     &          &          &          &          &          &          & $(0.07)$     & $(0.06)$     \\
Inequality level (t)          &              & $-0.07$  &          &          &          &          & $-0.05$  & $0.00$       & $0.02$       \\
                              &              & $(0.28)$ &          &          &          &          & $(0.28)$ & $(0.12)$     & $(0.12)$     \\
Unemployment (t)              &              &          & $0.36$   &          &          &          &          & $0.03$       & $0.05$       \\
                              &              &          & $(0.43)$ &          &          &          &          & $(0.29)$     & $(0.28)$     \\
Spatial EP (t)                &              &          &          & $0.12$   &          &          &          & $0.04$       & $0.04$       \\
                              &              &          &          & $(0.07)$ &          &          &          & $(0.04)$     & $(0.04)$     \\
Ed. Attainment (t)            &              &          &          &          & $-0.05$  &          &          &              & $0.12$       \\
                              &              &          &          &          & $(0.25)$ &          &          &              & $(0.12)$     \\
Log of personal Income PC (t) &              &          &          &          &          & $-0.09$  & $-0.09$  & $-0.05$      & $-0.09^{*}$  \\
                              &              &          &          &          &          & $(0.10)$ & $(0.10)$ & $(0.05)$     & $(0.05)$     \\
Log of GDP PC (t)             & $0.01$       & $-0.02$  & $-0.01$  & $0.02$   & $-0.01$  & $0.04$   & $0.04$   & $0.05$       & $0.06$       \\
                              & $(0.02)$     & $(0.04)$ & $(0.05)$ & $(0.06)$ & $(0.07)$ & $(0.08)$ & $(0.08)$ & $(0.04)$     & $(0.04)$     \\
Log of Pop. Density (t)       & $-0.00$      & $0.01$   & $0.01$   & $0.01$   & $0.01$   & $0.01$   & $0.01$   & $-0.00$      & $-0.00$      \\
                              & $(0.00)$     & $(0.01)$ & $(0.01)$ & $(0.01)$ & $(0.01)$ & $(0.01)$ & $(0.01)$ & $(0.00)$     & $(0.00)$     \\
\hline
Num. obs.                     & $250$        & $300$    & $300$    & $300$    & $300$    & $300$    & $300$    & $250$        & $250$        \\
R$^2$ (full model)            & $0.55$       & $0.03$   & $0.03$   & $0.10$   & $0.03$   & $0.03$   & $0.03$   & $0.55$       & $0.56$       \\
R$^2$ (proj model)            & $0.55$       & $0.03$   & $0.03$   & $0.10$   & $0.03$   & $0.03$   & $0.03$   & $0.55$       & $0.56$       \\
Adj. R$^2$ (full model)       & $0.53$       & $0.00$   & $0.00$   & $0.08$   & $-0.00$  & $0.01$   & $0.00$   & $0.53$       & $0.53$       \\
Adj. R$^2$ (proj model)       & $0.53$       & $-0.00$  & $0.00$   & $0.07$   & $-0.00$  & $0.01$   & $0.00$   & $0.53$       & $0.53$       \\
Num. groups: year             & $5$          & $6$      & $6$      & $6$      & $6$      & $6$      & $6$      & $5$          & $5$          \\
\hline
\multicolumn{10}{l}{\scriptsize{$^{***}p<0.01$; $^{**}p<0.05$; $^{*}p<0.1$}}
\end{tabular}
\caption{State-level regression analyses of EP as dependent variable. Each regression includes period-fixed effects. Standard errors in brackets. Note: ***$p<0.01$, **$p<0.05$, *$p<0.1$.}
\label{tab:epi_2}
\end{center}
\end{table}
