# Supplementary material for: Mapping Election Polarization and Competitiveness using Election Results
Source: arXiv:2308.10862 source file (2024-07-27)
Supplement: Supplementary file 5 [file EPI-v2.tex]

\begin{table}
\begin{center}
\begin{tabular}{l c c c c c c c c}
\hline
 & Model 1 & Model 2 & Model 3 & Model 4 & Model 5 & Model 6 & Model 7 & Model 8 \\
\hline
Inequality level (t - 1)          & $-0.38^{*}$  &              &              &              &              & $-0.36^{*}$  & $-0.49^{**}$ & $-0.46^{**}$ \\
                                  & $(0.22)$     &              &              &              &              & $(0.21)$     & $(0.21)$     & $(0.21)$     \\
Unemployment (t - 1)              &              & $0.71$       &              &              &              &              & $1.08$       & $1.12^{*}$   \\
                                  &              & $(0.56)$     &              &              &              &              & $(0.66)$     & $(0.66)$     \\
Spatial EP (t - 1)                &              &              & $0.07$       &              &              &              & $0.09$       & $0.09$       \\
                                  &              &              & $(0.07)$     &              &              &              & $(0.06)$     & $(0.06)$     \\
Spatial EP (t - 1)                &              &              & $0.07$       &              &              &              & $0.09$       & $0.09$       \\
                                  &              &              & $(0.07)$     &              &              &              & $(0.06)$     & $(0.06)$     \\
Ed. Attainment (t - 1)            &              &              &              & $0.01$       &              &              &              & $0.24$       \\
                                  &              &              &              & $(0.15)$     &              &              &              & $(0.25)$     \\
Log of personal Income PC (t - 1) &              &              &              &              & $-0.05$      & $-0.04$      & $0.03$       & $-0.02$      \\
                                  &              &              &              &              & $(0.06)$     & $(0.05)$     & $(0.07)$     & $(0.10)$     \\
Log of GDP PC (t - 1)             & $0.05^{***}$ & $0.04^{***}$ & $0.04^{***}$ & $0.04^{***}$ & $0.04^{***}$ & $0.05^{***}$ & $0.04^{***}$ & $0.04^{***}$ \\
                                  & $(0.01)$     & $(0.01)$     & $(0.01)$     & $(0.01)$     & $(0.01)$     & $(0.01)$     & $(0.01)$     & $(0.01)$     \\
Log of Pop. Density (t - 1)       & $-0.02^{**}$ & $-0.01$      & $-0.01^{*}$  & $-0.01$      & $-0.01$      & $-0.01^{*}$  & $-0.02^{**}$ & $-0.02^{**}$ \\
                                  & $(0.01)$     & $(0.01)$     & $(0.01)$     & $(0.01)$     & $(0.01)$     & $(0.01)$     & $(0.01)$     & $(0.01)$     \\
\hline
Num. obs.                         & $250$        & $250$        & $250$        & $250$        & $250$        & $250$        & $250$        & $250$        \\
R$^2$ (full model)                & $0.26$       & $0.25$       & $0.27$       & $0.24$       & $0.25$       & $0.27$       & $0.32$       & $0.33$       \\
R$^2$ (proj model)                & $0.26$       & $0.25$       & $0.27$       & $0.24$       & $0.25$       & $0.27$       & $0.32$       & $0.33$       \\
Adj. R$^2$ (full model)           & $0.24$       & $0.23$       & $0.25$       & $0.22$       & $0.22$       & $0.24$       & $0.29$       & $0.30$       \\
Adj. R$^2$ (proj model)           & $0.24$       & $0.23$       & $0.25$       & $0.21$       & $0.22$       & $0.24$       & $0.29$       & $0.29$       \\
Num. groups: year                 & $5$          & $5$          & $5$          & $5$          & $5$          & $5$          & $5$          & $5$          \\
\hline
\multicolumn{9}{l}{\scriptsize{$^{***}p<0.01$; $^{**}p<0.05$; $^{*}p<0.1$}}
\end{tabular}
\caption{State-level regression analyses of EP as dependent variable. Each regression includes period-fixed effects. Standard errors in brackets. Note: ***$p<0.01$, **$p<0.05$, *$p<0.1$.}
\label{tab:epi_3}
\end{center}
\end{table}
