# Supplementary material for: Mapping Election Polarization and Competitiveness using Election Results
Source: arXiv:2308.10862 source file (2024-07-27)
Supplement: Supplementary file 6 [file EPI.tex]

\begin{table}
\begin{center}
\begin{tabular}{l c c c c c c c c c}
\hline
 & Model 1 & Model 2 & Model 3 & Model 4 & Model 5 & Model 6 & Model 7 & Model 8 & Model 9 \\
\hline
EP (t - 1)                        & $0.64^{***}$ &              &              &              &              &              &              & $0.61^{***}$ & $0.61^{***}$ \\
                                  & $(0.06)$     &              &              &              &              &              &              & $(0.08)$     & $(0.07)$     \\
Inequality level (t - 1)          &              & $-0.38^{*}$  &              &              &              &              & $-0.36^{*}$  & $-0.14$      & $-0.11$      \\
                                  &              & $(0.22)$     &              &              &              &              & $(0.21)$     & $(0.10)$     & $(0.10)$     \\
Unemployment (t - 1)              &              &              & $0.71$       &              &              &              &              & $0.84^{*}$   & $0.89^{**}$  \\
                                  &              &              & $(0.56)$     &              &              &              &              & $(0.43)$     & $(0.44)$     \\
Spatial EP (t - 1)                &              &              &              & $0.07$       &              &              &              & $0.03$       & $0.03$       \\
                                  &              &              &              & $(0.07)$     &              &              &              & $(0.04)$     & $(0.04)$     \\
Spatial EP (t - 1)                &              &              &              & $0.07$       &              &              &              & $0.03$       & $0.03$       \\
                                  &              &              &              & $(0.07)$     &              &              &              & $(0.04)$     & $(0.04)$     \\
Ed. Attainment (t - 1)            &              &              &              &              & $0.01$       &              &              &              & $0.25^{*}$   \\
                                  &              &              &              &              & $(0.15)$     &              &              &              & $(0.13)$     \\
Log of personal Income PC (t - 1) &              &              &              &              &              & $-0.05$      & $-0.04$      & $0.02$       & $-0.04$      \\
                                  &              &              &              &              &              & $(0.06)$     & $(0.05)$     & $(0.04)$     & $(0.04)$     \\
Log of GDP PC (t - 1)             & $0.02^{**}$  & $0.05^{***}$ & $0.04^{***}$ & $0.04^{***}$ & $0.04^{***}$ & $0.04^{***}$ & $0.05^{***}$ & $0.01^{**}$  & $0.01^{**}$  \\
                                  & $(0.01)$     & $(0.01)$     & $(0.01)$     & $(0.01)$     & $(0.01)$     & $(0.01)$     & $(0.01)$     & $(0.01)$     & $(0.01)$     \\
Log of Pop. Density (t - 1)       & $-0.01^{**}$ & $-0.02^{**}$ & $-0.01$      & $-0.01^{*}$  & $-0.01$      & $-0.01$      & $-0.01^{*}$  & $-0.01^{**}$ & $-0.01^{**}$ \\
                                  & $(0.00)$     & $(0.01)$     & $(0.01)$     & $(0.01)$     & $(0.01)$     & $(0.01)$     & $(0.01)$     & $(0.01)$     & $(0.00)$     \\
\hline
Num. obs.                         & $250$        & $250$        & $250$        & $250$        & $250$        & $250$        & $250$        & $250$        & $250$        \\
R$^2$ (full model)                & $0.57$       & $0.26$       & $0.25$       & $0.27$       & $0.24$       & $0.25$       & $0.27$       & $0.59$       & $0.60$       \\
R$^2$ (proj model)                & $0.57$       & $0.26$       & $0.25$       & $0.27$       & $0.24$       & $0.25$       & $0.27$       & $0.59$       & $0.60$       \\
Adj. R$^2$ (full model)           & $0.56$       & $0.24$       & $0.23$       & $0.25$       & $0.22$       & $0.22$       & $0.24$       & $0.57$       & $0.58$       \\
Adj. R$^2$ (proj model)           & $0.56$       & $0.24$       & $0.23$       & $0.25$       & $0.21$       & $0.22$       & $0.24$       & $0.57$       & $0.57$       \\
Num. groups: year                 & $5$          & $5$          & $5$          & $5$          & $5$          & $5$          & $5$          & $5$          & $5$          \\
\hline
\multicolumn{10}{l}{\scriptsize{$^{***}p<0.01$; $^{**}p<0.05$; $^{*}p<0.1$}}
\end{tabular}
\caption{State-level regression analyses of EP as dependent variable. Each regression includes period-fixed effects. Standard errors in brackets. Note: ***$p<0.01$, **$p<0.05$, *$p<0.1$.}
\label{tab:epi_1}
\end{center}
\end{table}
