# Supplementary material for: Mapping Election Polarization and Competitiveness using Election Results
Source: arXiv:2308.10862 source file (2024-07-27)
Supplement: Supplementary file 7 [file Within-EPI-current.tex]

\begin{table}
\begin{center}
\begin{tabular}{l c c c c c c c c c}
\hline
 & Model 1 & Model 2 & Model 3 & Model 4 & Model 5 & Model 6 & Model 7 & Model 8 & Model 9 \\
\hline
Within-EP (t - 1)             & $1.02^{***}$ &          &          &              &          &               &               & $1.00^{***}$ & $0.99^{***}$ \\
                              & $(0.02)$     &          &          &              &          &               &               & $(0.02)$     & $(0.02)$     \\
Inequality level (t)          &              & $0.16$   &          &              &          &               & $0.25$        & $-0.06$      & $-0.06$      \\
                              &              & $(0.24)$ &          &              &          &               & $(0.23)$      & $(0.04)$     & $(0.04)$     \\
Unemployment (t)              &              &          & $0.29$   &              &          &               &               & $-0.12$      & $-0.11$      \\
                              &              &          & $(0.52)$ &              &          &               &               & $(0.10)$     & $(0.10)$     \\
Spatial Within-EP (t)         &              &          &          & $0.52^{***}$ &          &               &               & $0.06^{**}$  & $0.07^{**}$  \\
                              &              &          &          & $(0.13)$     &          &               &               & $(0.03)$     & $(0.03)$     \\
Ed. Attainment (t)            &              &          &          &              & $-0.20$  &               &               &              & $0.02$       \\
                              &              &          &          &              & $(0.22)$ &               &               &              & $(0.04)$     \\
Log of personal Income PC (t) &              &          &          &              &          & $-0.35^{***}$ & $-0.37^{***}$ & $-0.02$      & $-0.03$      \\
                              &              &          &          &              &          & $(0.12)$      & $(0.12)$      & $(0.02)$     & $(0.02)$     \\
Log of GDP PC (t)             & $-0.00$      & $-0.01$  & $-0.00$  & $0.06$       & $0.02$   & $0.22^{***}$  & $0.23^{***}$  & $0.02$       & $0.02$       \\
                              & $(0.01)$     & $(0.04)$ & $(0.04)$ & $(0.04)$     & $(0.04)$ & $(0.08)$      & $(0.08)$      & $(0.01)$     & $(0.01)$     \\
Log of Pop. Density (t)       & $-0.00^{**}$ & $0.00$   & $0.00$   & $-0.00$      & $0.00$   & $0.01$        & $0.01^{*}$    & $-0.00$      & $-0.00$      \\
                              & $(0.00)$     & $(0.01)$ & $(0.01)$ & $(0.01)$     & $(0.01)$ & $(0.01)$      & $(0.01)$      & $(0.00)$     & $(0.00)$     \\
\hline
Num. obs.                     & $250$        & $300$    & $300$    & $300$        & $300$    & $300$         & $300$         & $250$        & $250$        \\
R$^2$ (full model)            & $0.92$       & $0.18$   & $0.18$   & $0.33$       & $0.19$   & $0.28$        & $0.30$        & $0.93$       & $0.93$       \\
R$^2$ (proj model)            & $0.91$       & $0.01$   & $0.00$   & $0.19$       & $0.01$   & $0.13$        & $0.15$        & $0.91$       & $0.91$       \\
Adj. R$^2$ (full model)       & $0.92$       & $0.16$   & $0.16$   & $0.31$       & $0.16$   & $0.26$        & $0.28$        & $0.92$       & $0.92$       \\
Adj. R$^2$ (proj model)       & $0.91$       & $-0.02$  & $-0.02$  & $0.17$       & $-0.01$  & $0.11$        & $0.12$        & $0.91$       & $0.91$       \\
Num. groups: year             & $5$          & $6$      & $6$      & $6$          & $6$      & $6$           & $6$           & $5$          & $5$          \\
\hline
\multicolumn{10}{l}{\scriptsize{$^{***}p<0.01$; $^{**}p<0.05$; $^{*}p<0.1$}}
\end{tabular}
\caption{State-level regression analyses of Within-EP as dependent variable. Each regression includes period-fixed effects. Standard errors in brackets. Note: ***$p<0.01$, **$p<0.05$, *$p<0.1$.}
\label{tab:within_epi_2}
\end{center}
\end{table}
