# Supplementary material for: Mapping Election Polarization and Competitiveness using Election Results
Source: arXiv:2308.10862 source file (2024-07-27)
Supplement: Supplementary file 8 [file Within-EPI-v2.tex]

\begin{table}
\begin{center}
\begin{tabular}{l c c c c c c c c}
\hline
 & Model 1 & Model 2 & Model 3 & Model 4 & Model 5 & Model 6 & Model 7 & Model 8 \\
\hline
Inequality level (t - 1)          & $-0.21$      &              &              &              &              & $-0.16$      & $-0.24$       & $-0.22$       \\
                                  & $(0.21)$     &              &              &              &              & $(0.21)$     & $(0.21)$      & $(0.21)$      \\
Unemployment (t - 1)              &              & $0.14$       &              &              &              &              & $-0.02$       & $0.06$        \\
                                  &              & $(0.53)$     &              &              &              &              & $(0.52)$      & $(0.49)$      \\
Spatial Within-EP (t - 1)         &              &              & $0.34^{***}$ &              &              &              & $0.31^{**}$   & $0.36^{***}$  \\
                                  &              &              & $(0.12)$     &              &              &              & $(0.14)$      & $(0.14)$      \\
Ed. Attainment (t - 1)            &              &              &              & $-0.15$      &              &              &               & $0.27$        \\
                                  &              &              &              & $(0.17)$     &              &              &               & $(0.20)$      \\
Log of personal Income PC (t - 1) &              &              &              &              & $-0.10^{*}$  & $-0.10^{*}$  & $-0.04$       & $-0.09$       \\
                                  &              &              &              &              & $(0.05)$     & $(0.05)$     & $(0.07)$      & $(0.08)$      \\
Log of GDP PC (t - 1)             & $0.04^{***}$ & $0.04^{***}$ & $0.04^{***}$ & $0.04^{***}$ & $0.04^{***}$ & $0.04^{***}$ & $0.04^{***}$  & $0.04^{***}$  \\
                                  & $(0.01)$     & $(0.01)$     & $(0.01)$     & $(0.01)$     & $(0.01)$     & $(0.01)$     & $(0.01)$      & $(0.01)$      \\
Log of Pop. Density (t - 1)       & $-0.02^{**}$ & $-0.02^{**}$ & $-0.02^{**}$ & $-0.02^{**}$ & $-0.02^{**}$ & $-0.02^{**}$ & $-0.02^{***}$ & $-0.02^{***}$ \\
                                  & $(0.01)$     & $(0.01)$     & $(0.01)$     & $(0.01)$     & $(0.01)$     & $(0.01)$     & $(0.01)$      & $(0.01)$      \\
\hline
Num. obs.                         & $250$        & $250$        & $250$        & $250$        & $250$        & $250$        & $250$         & $250$         \\
R$^2$ (full model)                & $0.38$       & $0.37$       & $0.44$       & $0.38$       & $0.41$       & $0.42$       & $0.45$        & $0.47$        \\
R$^2$ (proj model)                & $0.28$       & $0.28$       & $0.35$       & $0.28$       & $0.32$       & $0.32$       & $0.37$        & $0.38$        \\
Adj. R$^2$ (full model)           & $0.36$       & $0.35$       & $0.42$       & $0.36$       & $0.39$       & $0.40$       & $0.43$        & $0.44$        \\
Adj. R$^2$ (proj model)           & $0.26$       & $0.25$       & $0.33$       & $0.26$       & $0.30$       & $0.30$       & $0.34$        & $0.35$        \\
Num. groups: year                 & $5$          & $5$          & $5$          & $5$          & $5$          & $5$          & $5$           & $5$           \\
\hline
\multicolumn{9}{l}{\scriptsize{$^{***}p<0.01$; $^{**}p<0.05$; $^{*}p<0.1$}}
\end{tabular}
\caption{State-level regression analyses of Within-EP as dependent variable. Each regression includes period-fixed effects. Standard errors in brackets. Note: ***$p<0.01$, **$p<0.05$, *$p<0.1$.}
\label{tab:within_epi_3}
\end{center}
\end{table}
