# Supplementary material for: Mapping Election Polarization and Competitiveness using Election Results
Source: arXiv:2308.10862 source file (2024-07-27)
Supplement: Supplementary file 10 [file polarization-manuscript.tex]

===============================================================================================================================================================
                          Model 1    Model 2    Model 3    Model 4     Model 5    Model 6     Model 7     Model 8     Model 9   Model 10  Model 11   Model 12  
---------------------------------------------------------------------------------------------------------------------------------------------------------------
Inequality level (t)       -0.02                  0.01       0.08       -0.02                   0.02        0.05       -0.00               -0.01       0.06    
                           (0.07)                (0.07)     (0.08)      (0.03)                 (0.03)      (0.04)      (0.06)              (0.07)     (0.07)   
Unemployment (t)                      -0.11 **   -0.12 **   -0.11 **               -0.16 ***   -0.17 ***   -0.09 **               0.03      0.03      -0.05    
                                      (0.04)     (0.04)     (0.05)                 (0.03)      (0.03)      (0.04)                (0.04)    (0.04)     (0.05)   
Polarization (t - 1)                                         0.22 ***                                       0.43 ***                                   0.19 ***
                                                            (0.08)                                         (0.07)                                     (0.05)   
Spatial polarization (t)                                     1.23 ***                                       0.49 ***                                   1.45 ***
                                                            (0.36)                                         (0.12)                                     (0.23)   
Ed. Attainment (t)         -0.05      -0.01      -0.00       0.15        0.27 **    0.33 ***    0.35 ***    0.07       -0.29 *   -0.30 *   -0.30 **    0.11    
                           (0.17)     (0.17)     (0.17)     (0.18)      (0.13)     (0.11)      (0.12)      (0.11)      (0.15)    (0.16)    (0.15)     (0.16)   
Personal Income PC (t)      0.01       0.06       0.05      -0.00        0.25 **    0.33 ***    0.31 ***   -0.02       -0.21 *   -0.23 *   -0.22 *    -0.05    
                           (0.14)     (0.14)     (0.14)     (0.14)      (0.10)     (0.09)      (0.09)      (0.12)      (0.11)    (0.12)    (0.12)     (0.14)   
GDP PC (t)                  0.23 **    0.15       0.15      -0.06        0.08      -0.03       -0.03        0.05        0.15      0.17      0.17      -0.08    
                           (0.09)     (0.09)     (0.10)     (0.11)      (0.08)     (0.08)      (0.08)      (0.07)      (0.11)    (0.11)    (0.11)     (0.12)   
Pop. Density (t)           -0.64      -0.56      -0.59      -1.53        0.04       0.18        0.11       -1.29 **    -0.65     -0.69     -0.66      -0.34    
                           (1.09)     (1.10)     (1.08)     (1.00)      (0.72)     (0.69)      (0.70)      (0.56)      (1.02)    (1.05)    (1.02)     (1.12)   
---------------------------------------------------------------------------------------------------------------------------------------------------------------
Num. obs.                 300        300        300        250         300        300         300         250         300       300       300        250       
R^2 (full model)            0.68       0.68       0.68       0.75        0.88       0.89        0.89        0.94        0.69      0.70      0.70       0.80    
R^2 (proj model)            0.02       0.04       0.04       0.14        0.55       0.59        0.59        0.73        0.25      0.25      0.25       0.44    
Adj. R^2 (full model)       0.60       0.61       0.61       0.67        0.85       0.87        0.87        0.93        0.63      0.63      0.63       0.74    
Adj. R^2 (proj model)      -0.20      -0.18      -0.18      -0.12        0.45       0.50        0.50        0.64        0.08      0.08      0.08       0.27    
Num. groups: state         50         50         50         50          50         50          50          50          50        50        50         50       
===============================================================================================================================================================
*** p < 0.01; ** p < 0.05; * p < 0.1
